# Supplementary material for: A Curriculum Domain Adaptation Approach to the Semantic Segmentation of Urban Scenes
Source: arXiv:1812.09953 source file (2019-01-10)
Supplement: Supplementary file 1 [file appendice.tex]

%!Tex root = main.tex

\section{Implementation Details}

\subsection{Hyper-parameters}

\section{Implemented Network Architecture}

\subsection{FCN-8s}

\subsection{ADEMXAPP}
